# Supplementary material for: Wukong: A Scalable and Locality-Enhanced Framework for Serverless Parallel Computing
Source: arXiv:2010.07268 source file (2020-10-14)
Supplement: Supplementary file 1 [file appendix.tex]

%\appendix
\begin{appendices}

\vspace{-6pt}
\section{Sensitivity Analysis}
\label{sec:sensitivity}
\vspace{-3pt}

In this Appendix section, we discuss the results of our sensitivity analysis of {\proj}. 

\begin{figure}[h]
\begin{center}
\includegraphics[width=0.38\textwidth]{Plots_v3/SVD2_PartitionSizeVsRuntime.pdf}
\caption{
SVD2 execution time as a function of the partition size.
}
\vspace{-10pt}
\label{fig:svd2-partitions-vs-runtime}
\end{center}
\end{figure}

\noindent\textbf{Partition Size.} 
The partition size of input data is one of the most important configuration parameters when executing a workload on {\proj}. This parameter controls how the input data is divided and subsequently processed, and presents an interesting tradeoff. Specifying a large partition size results in less parallelism and high network bandwidth consumption.
On the other hand, specifying a small partition size may generate too many fine-grained tasks, resulting in a very large number of individual connections between Task Executors and the storage cluster as well as very small data sizes for network I/O operations. Consequently, it is necessary for the user to find a balance in order to achieve optimal performance. The optimal value of the partition size will change depending on the application type and problem size. 

\begin{figure}[h]
\begin{center}
\includegraphics[width=0.4\textwidth]{Plots_v3/SVD2_NumFargateNodesVsRuntime.pdf}
\caption{
SVD2 performance and the I/O latencies when varying the Fargate cluster size.
}
\vspace{-15pt}
\label{fig:svd2-fargate-nodes-vs-runtime}
\end{center}
\end{figure}

Figure~\ref{fig:svd2-partitions-vs-runtime} shows the performance of SVD2 with a problem size of \(50k \times 50k\) for various partition sizes. Selecting a small partition size such as \(2k \times 2k\) causes significant network contention resulting from too many individual connections and I/O operations. Increasing the partition size alleviates this contention and improves overall performance. Notice that continuing to increase the problem size for SVD2 does not impact performance significantly. Instead, the performance will remain approximately the same as the partition size increases.  This is because task clustering and delayed I/O prevent network communication of large objects. That is, increasing the partition size does not impact the workload significantly once clustering and delay I/O are in effect.

\noindent\textbf{Number of Storage Nodes.} Next, we evaluate how the number of nodes in the storage substrate impacts execution time. Figure~\ref{fig:svd2-fargate-nodes-vs-runtime} shows the performance of SVD2 with a problem size of \(128k \times 128k\) for different numbers of Fargate nodes, along with the associated average read and write latencies for each configuration. Using a small number of nodes such as 5 or 10 results in significant performance degradation, as the limited number of Redis instances suffer severe network bandwidth contention. As we increase the size of the Fargate cluster, read latencies decrease significantly, resulting in a lower execution time for the workload.

Execution time will no longer decrease once the number of Fargate nodes increases beyond a certain threshold. The value of this threshold is predominantly dependent on problem size, as a larger problem size would benefit from a larger number of Fargate nodes compared to a smaller problem size. 

\newpage

\section{Benchmark Code Snippets and DAGs}
\label{sec:appendix-codes}

In this Appendix section, we list the code snippet for each benchmark that we used along with exemplar DAG generated under small problem size (for visibility and illustration purpose).

\begin{figure}[ht]
  \begin{subfigure}{Code:}
    \begin{minted}[fontsize=\footnotesize, xleftmargin=5pt, numbersep=1pt,linenos]{python}
  X = da.random.random((8_192_000, 100), 
                       chunks=(10000, 100))
  u, s, v = da.linalg.svd_compressed(X, k=5)
  res = c.compute(v)
    \end{minted}
  \end{subfigure}
  \begin{subfigure}{DAG for illustration: 10x2, chunks=(5x2) }
    \begin{center}
    \includegraphics[width=.25\textwidth]{DAGs/SVD1 10 x 2 (chunks = 5 x 2).pdf}
    \end{center}
  \end{subfigure}
  \caption{\label{fig:svd1} The DAG of tall-and-skinny SVD (SVD1).}
  \vspace{-0.05in}
\end{figure}

\begin{figure}[ht]
  \begin{subfigure}{Code:}
    \begin{minted}[fontsize=\footnotesize, xleftmargin=5pt, numbersep=1pt,linenos]{python}
  X = da.random.random((256_000, 256_000), 
                       chunks=(5000, 5000))
  u, s, v = da.linalg.svd_compressed(X, k=5)
  res = c.compute(v)
    \end{minted}
  \end{subfigure}
  \begin{subfigure}{DAG for illustration: 200x200, chunks=(50x50) }
    \begin{center}
    \includegraphics[width=.5\textwidth]{DAGs/SVD2 200 x 200 chunks = 50 x 50.pdf}
    \end{center}
  \end{subfigure}
  \caption{\label{fig:svd2} The DAG of square SVD (SVD2).}
  \vspace{-0.05in}
\end{figure}

\begin{figure}[ht]
  \begin{subfigure}{Code:}
    \begin{minted}[fontsize=\footnotesize, xleftmargin=5pt, numbersep=1pt,linenos]{python}
  X = da.random.random((67_108_864, 128), 
                       chunks = (16384, 128))
  q, r = da.linalg.tsqr(X)
  res = r.compute()
    \end{minted}
  \end{subfigure}
  \begin{subfigure}{DAG for illustration: 32768x128, chunks=(8192x128) }
    \includegraphics[width=.5\textwidth]{DAGs/TSQR 32768 x 128 (8192 x 128).pdf}
  \end{subfigure}
  \caption{\label{fig:tsqr} DAG of tall-and-skinny QR factorization (TSQR).}
  \vspace{-0.05in}
\end{figure}

\begin{comment}
\begin{figure}[ht]
  \begin{subfigure}{Code:}
    \begin{minted}[fontsize=\footnotesize, xleftmargin=5pt, numbersep=1pt,linenos]{python}
  def get_sym(input_size, _chunks):
    A = da.ones((input_size,input_size),
                chunks = _chunks)
    lA = da.tril(A)
    return lA.dot(lA.T)

  X = get_sym(25000, _chunks = (2000, 2000))
  chol = da.linalg.cholesky(X)
  res = chol.compute()
    \end{minted}
  \end{subfigure}
  \begin{subfigure}{DAG for illustration: 200x200, chunks=(50x50) }
    \includegraphics[width=.5\textwidth]{DAGs/Cholesky 200 x 200 (50 x 50).pdf}
  \end{subfigure}
  \caption{\label{fig:cholesky} Benchmark for Cholesky Decomposition}
  \vspace{-0.05in}
\end{figure}
\end{comment}

\begin{figure}[ht]
    \begin{subfigure}{Code:}
        \begin{minted}[fontsize=\footnotesize, xleftmargin=5pt, numbersep=1pt,linenos]{python}
  X = da.random.random((25_000, 25_000), 
                       chunks = (2000, 2000))
  Y = da.random.random((25_000, 25_000), 
                       chunks = (2000, 2000))
  z = da.matmul(X, Y)
  z.compute()
        \end{minted}
    \end{subfigure}
    \begin{subfigure}{DAG for illustration: 10x10, chunks=(5x5) }
        \begin{center}
        \includegraphics[width=.5\textwidth]{DAGs/GEMM 10 x 10 (chunks = 5 x 5).pdf}
        \end{center}
    \end{subfigure}
\caption{\label{fig:gemm} DAG of GEMM.}
\vspace{-0.05in}
\end{figure}

\begin{figure}[ht]
  \begin{subfigure}{Code:}
    \begin{minted}[fontsize=\footnotesize, xleftmargin=5pt, numbersep=1pt,linenos]{python}
  X,Y = sklearn.datasets.make_classification(n_samples=1000)
  clf = ParallelPostFit(SVC(gamma='scale'))
  clf.fit(X, Y)

  X,Y = dask_ml.datasets.make_classification(
          n_samples = 32_768_000,
          random_state = 32_768_000,
          chunks = 32_768_000 // 160)
  ans = clf.predict(X).compute()
    \end{minted}
  \end{subfigure}
  \begin{subfigure}{DAG for illustration: n=100, chunks=20 }
    \includegraphics[width=.5\textwidth]{DAGs/SVC n = 100, chunks = 20.pdf}
  \end{subfigure}
  \caption{\label{fig:svc} DAG of SVC.}
  \vspace{-0.05in}
\end{figure}

\begin{figure}[ht]
  \begin{subfigure}{Code:}
    \begin{minted}[fontsize=\footnotesize, xleftmargin=5pt, numbersep=1pt,linenos]{python}
  def add(x,y):
    time.sleep(0.5)
    return x + y

  L = range(1024)
  while len(L) > 1:
    L = list(map(delayed(add), L[0::2], L[1::2]))

  L[0].compute()
    \end{minted}
  \end{subfigure}
  \begin{subfigure}{DAG for illustration: len(L)=8 }
    \includegraphics[width=.5\textwidth]{DAGs/Tree Reduction (N = 8).pdf}
  \end{subfigure}
  \caption{\label{fig:treereduction} DAG of tree reduction. }
  \vspace{-0.05in}
\end{figure}

\end{appendices}
